# Supplementary material for: Spatially-resolved dynamics of the amplitude Schmid-Higgs mode in disordered superconductors
Source: arXiv:2409.11647 source file (2025-08-05)
Supplement: Supplementary file 1 [file SM.pdf]

# ONLINE SUPPORTING INFORMATION

## Spatially-resolved dynamics of the amplitude Schmid-Higgs mode in disordered superconductors

P. A. Nosov,<sup>1</sup> E. S. Andriyakhina,<sup>2</sup> and I. S. Burmistrov<sup>3,4</sup>

<sup>1</sup>*Stanford Institute for Theoretical Physics, Stanford University, Stanford, CA 94305, USA*

<sup>2</sup>*Dahlem Center for Complex Quantum Systems and Physics Department,  
Freie Universität Berlin, Arnimallee 14, Berlin, 14195, Germany*

<sup>3</sup>*L.D. Landau Institute for Theoretical Physics, acad. Semenova av.1-a, Chernogolovka, 142432, Russia*

<sup>4</sup>*Laboratory for Condensed Matter Physics, HSE University, Moscow, 101000, Russia*

These notes contain: (i) derivation of the SH susceptibility on the Matsubara axis (Eq. (3) of the main text) and its analytic continuation to the physical Riemann sheet (Eq. (4) of the main text), (ii) derivation of the approximate expression for the retarded SH susceptibility in the dirty limit (Eq. (7) of the main text), and (iii) details of the long-distance and late-time asymptotic analysis of the SH response.

### DERIVATION OF THE SH SUSCEPTIBILITY

The normal and anomalous Matsubara Green's functions of a disordered BCS superconductor can be expressed in the exact eigenbasis defined for a given realization of random potential:

$$G(i\varepsilon_n, \mathbf{r}, \mathbf{r}') = \sum_{\alpha} \varphi_{\alpha}(\mathbf{r}) \varphi_{\alpha}(\mathbf{r}') \frac{i\varepsilon_n + \xi_{\alpha}}{\varepsilon_n^2 + \xi_{\alpha}^2 + \Delta^2}, \quad F(i\varepsilon_n, \mathbf{r}, \mathbf{r}') = \sum_{\alpha} \varphi_{\alpha}(\mathbf{r}) \varphi_{\alpha}(\mathbf{r}') \frac{\Delta}{\varepsilon_n^2 + \xi_{\alpha}^2 + \Delta^2}, \quad (\text{S1})$$

where  $\varepsilon_n = 2\pi T(n+1/2)$ , and  $\varphi_{\alpha}(\mathbf{r})$  is the exact single particle eigenfunction with the energy  $\xi_{\alpha}$ . The mean-field order parameter  $\Delta$  is determined via the self-consistency condition  $\Delta = \lambda_{\text{BCS}} T \sum_m F(\varepsilon_m, \mathbf{r}, \mathbf{r}') / \nu$ . The latter, according to the Anderson's theorem [1–3], leads to the standard BCS gap equation

$$1 = \pi \lambda_{\text{BCS}} T \sum_m \frac{1}{\sqrt{\Delta^2 + \varepsilon_m^2}}, \quad (\text{S2})$$

provided that the wave-function amplitude  $|\psi_{\alpha}(\mathbf{r})|^2$  is essentially a non-fluctuating constant set only by normalization. Within the mean-field approach,  $\Pi_{\Delta\Delta}$  can be computed as follows

$$\Pi_{\Delta\Delta}(i\omega_n, \mathbf{r}, \mathbf{r}') = \frac{T}{\pi\nu} \sum_m \left\{ G(i\varepsilon_m + i\omega_n, \mathbf{r}, \mathbf{r}') G(-i\varepsilon_m, \mathbf{r}, \mathbf{r}') - F(i\varepsilon_m + i\omega_n, \mathbf{r}, \mathbf{r}') F(-i\varepsilon_m, \mathbf{r}, \mathbf{r}') \right\} \quad (\text{S3})$$

Our first step is to calculate the disorder-averaged Fourier transform of this correlation function

$$\Pi_{\Delta\Delta}(i\omega_n, \mathbf{q}) \equiv \int d^d r' \overline{\Pi_{\Delta\Delta}(i\omega_n, \mathbf{r}, \mathbf{r}') e^{i\mathbf{q} \cdot (\mathbf{r} - \mathbf{r}')}}, \quad (\text{S4})$$

where  $\overline{A}$  denotes the average of  $A$  over different realizations of disorder. This average can be performed by using the well-known expression for the averaged irreducible dynamical structure factor of single-particle wave-functions in a random potential [4, 5]

$$\int d^d r' e^{i\mathbf{q} \cdot (\mathbf{r} - \mathbf{r}')} \sum_{\alpha\beta} \overline{\varphi_{\alpha}(\mathbf{r}) \varphi_{\beta}(\mathbf{r}) \varphi_{\alpha}(\mathbf{r}') \varphi_{\beta}(\mathbf{r}') \delta(\xi - \xi_{\alpha}) \delta(\xi' - \xi_{\beta})} = \frac{\nu}{2} \left[ S_{\mathbf{q}}(i(\xi - \xi')) + S_{\mathbf{q}}(i(\xi' - \xi)) \right]. \quad (\text{S5})$$

Here,  $S_{\mathbf{q}}(z)$  is the analytic continuation of the structure factor  $S_{\mathbf{q}}(E)$ , given in the main text, from real  $E > 0$  to complex  $z$ . In particular, in 2D and 3D we have

$$[S_{\mathbf{q}}^{2\text{D}}(E)]^{-1} = \sqrt{v_F^2 q^2 + (1/\tau + E)^2} - 1/\tau, \quad [S_{\mathbf{q}}^{3\text{D}}(E)]^{-1} = \frac{2iv_F q}{\ln[(1 + \tau E + ilq)/(1 + \tau E - ilq)]} - 1/\tau. \quad (\text{S6})$$

We emphasize that Eq. (S5) and Eq. (S6) are well-justified in the diffusive limit  $E_F \tau \gg 1$  and  $q \ll l$ , where  $l = v_F \tau$  is the mean free path,  $v_F$  is the Fermi velocity,  $\tau$  is the mean free time, and  $E_F$  is the Fermi energy. Diagrammatically,

this expression corresponds to the summation of the ladder-type corrections to the particle-hole and particle-particle propagators [6, 7]. As clearly seen from Eq. (S6),  $S_{\mathbf{q}}(iz)$  is analytic in the lower half-plane of  $z$ , whereas  $S_{\mathbf{q}}(-iz)$  is analytic in the upper half-plane.

After substituting Eq. (S1) into Eq. (S3), and using Eq. (S5) in combination with additional unity insertions  $1 = \int d\xi \delta(\xi - \xi_\alpha)$  under the sum, we obtain

$$\Pi_{\Delta\Delta}(i\omega_n, \mathbf{q}) = \frac{T}{2\pi} \sum_m \int_{-\infty}^{\infty} d\xi d\xi' \frac{(i\varepsilon_m + i\omega_n + \xi)(-i\varepsilon_m + \xi') - \Delta^2}{((\varepsilon_m + \omega_n)^2 + \xi^2 + \Delta^2)(\varepsilon_m^2 + \xi'^2 + \Delta^2)} \left[ S_{\mathbf{q}}(i(\xi - \xi')) + S_{\mathbf{q}}(i(\xi' - \xi)) \right]. \quad (\text{S7})$$

Let us first integrate over  $\xi$ . The poles of the prefactor are at  $\xi = \pm iE_{\varepsilon_m + \omega_n}$ , where  $E_\xi = \sqrt{\xi^2 + \Delta^2}$ . The first (second) term in square brackets has its non-analyticities at  $\text{Im } \xi > 0$  ( $\text{Im } \xi < 0$ ). Thus, for the first term we can close the contour of integration in the lower half-plane of  $\xi$  and pick up the residue at  $\xi = -iE_{\varepsilon_m + \omega_n}$ , and for the second term we close the contour in the upper half-plane. The remaining integral over  $\xi'$  can be done in the same way. We thus arrive at the following expression

$$\Pi_{\Delta\Delta}(i\omega_n, \mathbf{q}) = \pi T \sum_m S_{\mathbf{q}}(E_{\varepsilon_m} + E_{\varepsilon_m + \omega_n}) \left[ 1 + \frac{\varepsilon_m(\varepsilon_m + \omega_n) - \Delta^2}{E_{\varepsilon_m} E_{\varepsilon_m + \omega_n}} \right]. \quad (\text{S8})$$

After combining the definition of the inverse SH susceptibility (Eq. (2) from the main text), our result in Eq. (S8), and the gap equation Eq. (S2), we finally arrive at

$$\frac{1}{\chi_{\text{SH}}(i\omega_n, \mathbf{q})} = \pi T \sum_m \left\{ \frac{1}{E_{\varepsilon_m}} - S_{\mathbf{q}}(E_{\varepsilon_m} + E_{\varepsilon_m + |\omega_n|}) \left[ 1 + \frac{\varepsilon_m(\varepsilon_m + |\omega_n|) - \Delta^2}{E_{\varepsilon_m} E_{\varepsilon_m + |\omega_n|}} \right] \right\}, \quad (\text{S9})$$

where we also replaced  $\omega_n$  with  $|\omega_n|$  because the sum is an even function of  $\omega_n$ . Eq. (S9) is Eq. (2) of the main text. At  $q = 0$  and  $T = 0$ , this expression reduces to

$$\frac{1}{\chi_{\text{SH}}(i\omega_n, 0)} = \frac{\sqrt{4\Delta^2 + \omega_n^2}}{2|\omega_n|} \ln \left( \frac{\sqrt{4\Delta^2 + \omega_n^2} + |\omega_n|}{\sqrt{4\Delta^2 + \omega_n^2} - |\omega_n|} \right). \quad (\text{S10})$$

We note that, strictly speaking, the r.h.s. in Eq. (S9) is the disorder-averaged inverse SH susceptibility, and not the inverse of the averaged SH susceptibility. However, the difference is a small correction of higher order in  $1/E_F\tau \ll 1$  which can be safely neglected [7].

### Analytic continuation on the physical Riemann sheet

Our next task is to analytically continue Eq. (S9) into a complex frequency plane on the physical Riemann sheet. First, we establish the relation between the desired analytic continuation  $\chi_{\text{SH}}(z, \mathbf{q})$  and the retarded function  $\chi_{\text{SH}}^R(\varepsilon, \mathbf{q}) \equiv \chi_{\text{SH}}(\varepsilon + i0^+, \mathbf{q})$  defined slightly above the real axis. Let us consider the following identity

$$\frac{1}{\chi_{\text{SH}}(i\omega_n, \mathbf{q})} = \int_{\mathcal{C}} \frac{dz}{2\pi i} \frac{[\chi_{\text{SH}}(z, \mathbf{q})]^{-1}}{z - i\omega_n}, \quad (\text{S11})$$

where  $\mathcal{C}$  is a small closed contour encircling  $i\omega_n$ , and  $\omega_n \geq 0$ . As guaranteed by causality, the desired analytic continuation  $[\chi_{\text{SH}}(z, \mathbf{q})]^{-1}$  is analytic in the upper half-plane  $\text{Im } z > 0$ . Thus, we can extend the contour to go slightly above the real axis from  $-\Lambda + i0^+$  to  $+\Lambda + i0^+$ ,  $\Lambda \rightarrow +\infty$ , and close it in the upper half-plane

$$\frac{1}{\chi_{\text{SH}}(i\omega_n, \mathbf{q})} = \lim_{\Lambda \rightarrow +\infty} \left\{ \int_{-\Lambda}^{+\Lambda} \frac{d\varepsilon}{2\pi i} \frac{[\chi_{\text{SH}}^R(\varepsilon, \mathbf{q})]^{-1}}{\varepsilon - i\omega_n} + \frac{\Lambda}{2\pi} \int_0^\pi d\theta \frac{e^{i\theta} [\chi_{\text{SH}}(\Lambda e^{i\theta}, \mathbf{q})]^{-1}}{\Lambda e^{i\theta} - i\omega_n} \right\}. \quad (\text{S12})$$

Normally, the second term vanishes in the limit  $\Lambda \rightarrow \infty$ , whereas the first term is finite and leads to the usual Kramers–Kronig-type relation. Here this is not the case: as one can see from Eq. (S10),  $1/|\chi_{\text{SH}}(i\omega_n, \mathbf{q})|$  is a growing

function on the Matsubara axis. As a consequence, both terms in Eq. (S12) diverge logarithmically. However, as we will see, their divergencies exactly compensate each other. Let us consider the second integral and approximate it as

$$\frac{\Lambda}{2\pi} \int_0^\pi d\theta \frac{e^{i\theta} [\chi_{\text{SH}}(\Lambda e^{i\theta}, \mathbf{q})]^{-1}}{\Lambda e^{i\theta} - i\omega_n} \approx \frac{1}{2\pi} \int_0^\pi d\theta [\chi_{\text{SH}}(\Lambda e^{i\theta}, \mathbf{q})]^{-1} + \mathcal{O}(\Lambda^{-1}). \quad (\text{S13})$$

Next, we can use the fact that the SH susceptibility becomes momentum-independent at large complex frequencies, so we can directly use the  $q = 0$  expression in Eq. (S10)

$$[\chi_{\text{SH}}(z = \Lambda e^{i\theta}, \mathbf{q})]^{-1} \approx [\chi_{\text{SH}}(z = \Lambda e^{i\theta}, 0)]^{-1} = \frac{i\sqrt{4\Delta^2 - z^2}}{2z} \ln \left( \frac{\sqrt{4\Delta^2 - z^2} - iz}{\sqrt{4\Delta^2 - z^2} + iz} \right) = -\frac{i\pi}{2} + i\theta + \ln \frac{\Lambda}{\Delta} + \mathcal{O}(\Lambda^{-1}). \quad (\text{S14})$$

After integrating over  $\theta$  and replacing  $\ln \Lambda/\Delta$  with the integral  $\frac{1}{2} \int_{-\Lambda}^\Lambda d\varepsilon \frac{\theta(|\varepsilon| - 2\Delta)}{\sqrt{\varepsilon^2 - 4\Delta^2}}$  (up to small corrections vanishing in the limit  $\Lambda \rightarrow \infty$ ), we obtain

$$\frac{1}{\chi_{\text{SH}}(i\omega_n, \mathbf{q})} = \int_{-\infty}^{+\infty} \frac{d\varepsilon}{2\pi} \left\{ \frac{\pi \theta(|\varepsilon| - 2\Delta)}{2\sqrt{\varepsilon^2 - 4\Delta^2}} - \frac{i[\chi_{\text{SH}}^R(\varepsilon, \mathbf{q})]^{-1}}{\varepsilon - i\omega_n} \right\}, \quad \omega_n \geq 0. \quad (\text{S15})$$

If  $i\omega_n$  is continued to complex frequency  $z$ , then the integral on the r.h.s. of the expression above gives  $1/\chi_{\text{SH}}(z, \mathbf{q})$  if  $\text{Im } z > 0$ , and zero if  $\text{Im } z < 0$  (this is evident from the r.h.s. of Eq. (S11) - the only non-analyticity of the integrand at  $z$  leaves the area that could be enclosed by  $\mathcal{C}$  without crossing the branch cut on the real axis). Evidently, since  $\chi_{\text{SH}}(i\omega_n, \mathbf{q}) = \chi_{\text{SH}}(-i|\omega_n|, \mathbf{q}) = \chi_{\text{SH}}(i|\omega_n|, \mathbf{q})$  for  $\omega_n < 0$ , we also have the following representation

$$\frac{1}{\chi_{\text{SH}}(i\omega_n, \mathbf{q})} = \int_{-\infty}^{+\infty} \frac{d\varepsilon}{2\pi} \left\{ \frac{\pi \theta(|\varepsilon| - 2\Delta)}{2\sqrt{\varepsilon^2 - 4\Delta^2}} - \frac{i[\chi_{\text{SH}}^R(\varepsilon, \mathbf{q})]^{-1}}{\varepsilon + i\omega_n} \right\}, \quad \omega_n < 0. \quad (\text{S16})$$

We again notice that after  $i\omega_n$  is replaced with  $z$ , the integral on the r.h.s. is identical to  $1/\chi_{\text{SH}}(z, \mathbf{q})$  if  $\text{Im } z < 0$ , and produces zero if  $\text{Im } z > 0$ . Thus, the integral representation of  $1/\chi_{\text{SH}}(z, \mathbf{q})$  in the entire complex plane (except for the branch cuts on the real axis) is given by the sum of integrals on the r.h.s. of Eq. (S15) and Eq. (S16) with  $i\omega_n$  replaced by  $z$

$$\frac{1}{\chi_{\text{SH}}(z, \mathbf{q})} = \int_{-\infty}^{+\infty} \frac{d\varepsilon}{2\pi} \left\{ \frac{\pi \theta(|\varepsilon| - 2\Delta)}{2\sqrt{\varepsilon^2 - 4\Delta^2}} - \frac{i[\chi_{\text{SH}}^R(\varepsilon, \mathbf{q})]^{-1}}{\varepsilon - z} - \frac{i[\chi_{\text{SH}}^R(\varepsilon, \mathbf{q})]^{-1}}{\varepsilon + z} \right\} = \int_{-\infty}^{+\infty} \frac{d\varepsilon}{\pi} \left\{ \frac{\text{Im}[\chi_{\text{SH}}^R(\varepsilon, \mathbf{q})]^{-1}}{\varepsilon - z} + \frac{\pi \theta(|\varepsilon| - 2\Delta)}{2\sqrt{\varepsilon^2 - 4\Delta^2}} \right\} \quad (\text{S17})$$

where we used the fact that the real (imaginary) part of  $[\chi_{\text{SH}}^R(\varepsilon, \mathbf{q})]^{-1}$  is even (odd). After rewriting  $\text{Im}[\chi_{\text{SH}}^R(\varepsilon, \mathbf{q})]^{-1}$  via the spectral density  $\rho_{\mathbf{q}}(\varepsilon)$  as  $\text{Im}[\chi_{\text{SH}}^R(\varepsilon, \mathbf{q})]^{-1} = \text{sgn}(\varepsilon)\theta(|\varepsilon| - 2\Delta)\rho_{\mathbf{q}}(|\varepsilon|)$ , we arrive at Eq. (4) of the main text.

The remaining step is to calculate  $\text{Im}[\chi_{\text{SH}}^R(\varepsilon, \mathbf{q})]^{-1}$  at  $T = 0$ . In principle, this can be done directly from (S9) by transforming the sum into a real-frequency integral involving the Fermi-Dirac distribution. Next,  $i\omega_n$  is replaced by  $\omega + i0^+$ , and the imaginary part is taken at  $T = 0$ . Here we take a slightly different route and start with Eq. (S7). After replacing the sum with an integral, we find

$$\Pi_{\Delta\Delta}(i\omega_n, \mathbf{q}) = \frac{1}{\pi} \int_{-\infty}^{\infty} d\xi d\xi' \text{Re} \{S_{\mathbf{q}}(i(\xi - \xi'))\} \int_{\mathcal{C}} \frac{dz}{4\pi i} \mathcal{F}(z) \frac{(z + i\omega_n + \xi)(\xi' - z) - \Delta^2}{(\xi^2 + \Delta^2 - (z + i\omega_n)^2)(\xi'^2 + \Delta^2 - z^2)}, \quad (\text{S18})$$

where  $\mathcal{F}(z) = \tanh(z/2T)$ , and the contour  $\mathcal{C}$  consists of small circles enclosing only the poles at  $z = i\varepsilon_m$  for  $m \in \mathbb{Z}$ . The other poles of the integrand are at  $\pm E_{\xi'}$  and  $-i\omega_n \pm E_{\xi}$ . After deforming the contour to infinity, we pick up the contributions from these poles, and find

$$\Pi_{\Delta\Delta}(i\omega_n, \mathbf{q}) = \sum_{\eta=\pm} \int_{-\infty}^{\infty} \frac{d\xi d\xi'}{4\pi} \text{Re} \{S_{\mathbf{q}}(i(\xi - \xi'))\} \mathcal{F}(E_{\xi}) \frac{(i\omega_n + \xi' - \eta E_{\xi})(\xi + \eta E_{\xi}) - \Delta^2}{E_{\xi} E_{\xi'}} \left[ \frac{1}{i\omega_n - \eta E_{\xi} + E_{\xi'}} - \frac{1}{i\omega_n - \eta E_{\xi} - E_{\xi'}} \right]. \quad (\text{S19})$$

Here we used  $\mathcal{F}(E - i\eta\omega_n) = \mathcal{F}(E)$ ,  $\mathcal{F}(-E) = \mathcal{F}(E)$ , and interchanged the integration variables  $\xi \leftrightarrow \xi'$  in one of the terms. For further convenience, we can use the following identity

$$1 = \int_{\Delta}^{+\infty} dE \delta(E - E_{\varepsilon}) = \int_{\Delta}^{+\infty} dE \sum_{s=\pm} \frac{E}{\sqrt{E^2 - \Delta^2}} \delta(\varepsilon + s\sqrt{E^2 - \Delta^2}) \quad (\text{S20})$$

in order to eliminate the integrals over  $\xi, \xi'$ . After setting  $T=0$  and taking the imaginary part of the resulting expression, we find

$$\begin{aligned} \text{Im} \Pi_{\Delta\Delta}^R(\omega, \mathbf{q}) &= \frac{1}{2} \sum_{\eta=\pm} \int_{\Delta}^{+\infty} dE dE' \left[ \eta + \frac{E(|\omega| - E) - \Delta^2}{\sqrt{E^2 - \Delta^2} \sqrt{E'^2 - \Delta^2}} \right] (\delta(\omega - E - E') - \delta(\omega + E + E')) \\ &\times \text{Re} S_{\mathbf{q}}(i(\sqrt{E^2 - \Delta^2} - \eta\sqrt{E'^2 - \Delta^2})). \end{aligned} \quad (\text{S21})$$

The final result reads as

$$\begin{aligned} \text{Im}[\chi_{\text{SH}}^R(\omega, \mathbf{q})]^{-1} &= -\frac{1}{2} \text{sgn}(\omega) \theta(|\omega| - 2\Delta) \sum_{\eta=\pm} \int_{\Delta}^{|\omega|-\Delta} dE \left[ \eta + \frac{E(|\omega| - E) - \Delta^2}{\sqrt{E^2 - \Delta^2} \sqrt{(|\omega| - E)^2 - \Delta^2}} \right] \\ &\times \text{Re} S_{\mathbf{q}}(i(\sqrt{E^2 - \Delta^2} - \eta\sqrt{(|\omega| - E)^2 - \Delta^2})). \end{aligned} \quad (\text{S22})$$

This expression is valid for arbitrary  $\Delta\tau$ . In the dirty limit,  $\Delta\tau \ll 1$ , the integral can be done analytically in terms of Elliptic functions, and the result is given in Eq. (5) of the main text.

Let us now demonstrate that Eq. (S22) reproduces the correct answer in the clean limit  $1/\tau = 0$ , in particular in two dimensions [8]. After setting  $1/\tau$  to zero in Eq. (S6), or evaluating Eq. (S5) directly by replacing random wave-functions with plane waves, we find  $\text{Re} S_{\mathbf{q}}(ix) = \theta(v_F q - |x|) / \sqrt{v_F^2 q^2 - x^2}$ . We substitute this expression in Eq. (S22) and expand the integrand in powers of  $v_F q / \Delta \ll 1$  and  $(\omega / \Delta - 2) \ll 1$  while keeping the ratio  $4\Delta^2(\omega / \Delta - 2) / (v_F^2 q^2) = \zeta$  fixed. For  $\zeta < 1$ , the step-function in Eq. (S22) equals to one for all  $E$ , and we obtain

$$\text{Im}[\chi_{\text{SH}}^R(\omega, \mathbf{q})]^{-1} = -\frac{v_F q}{2\Delta} \sqrt{\zeta} \text{Re} E \left( \frac{1}{\sqrt{\zeta + i0^+}} \right), \quad \omega > 2\Delta, \quad (\text{S23})$$

where  $0 < \zeta < 1$ , and  $E(x) = \int_0^{\pi/2} d\theta \sqrt{1 - x^2 \sin^2 \theta}$ . Eq. (S23) agrees with Eq. (21) in [8].

### REAL PART OF $\chi_{\text{SH}}^R$ IN THE DIRTY LIMIT $\Delta\tau \ll 1$

As was explained in the main text, the behavior of  $\text{Im} 1/\chi_{\text{SH}}^R(\omega, \mathbf{q})$  for  $\Delta\tau \ll 1$  and in the long-wavelength limit  $\xi q \ll 1$ ,  $|\omega - 2\Delta|/\Delta \ll 1$  with  $|\omega/\Delta - 2|/\xi^4 q^4$  fixed can be easily obtained by expanding our full analytic result in Eq. (5) of the main text. The real part of  $1/\chi_{\text{SH}}^R(\omega, \mathbf{q})$  is given by the principle value of the integral

$$\text{Re}[\chi_{\text{SH}}^R(\omega, \mathbf{q})]^{-1} = \oint_{-\infty}^{+\infty} \frac{d\varepsilon}{\pi} \left\{ \frac{\text{Im}[\chi_{\text{SH}}^R(\varepsilon, \mathbf{q})]^{-1}}{\varepsilon - \omega} + \frac{\pi \theta(|\varepsilon| - 2\Delta)}{2 \sqrt{\varepsilon^2 - 4\Delta^2}} \right\}. \quad (\text{S24})$$

This integral can be computed in two steps. First, we notice that  $\text{Re}[\chi_{\text{SH}}^R(2\Delta + 0^+, 0)]^{-1} = 0$ . This is most easily seen directly from Eq. (S10). Alternatively, one can take the  $q=0$  limit in Eq. (5) of the main text, yielding  $\text{Im}[\chi_{\text{SH}}^R(\omega, 0)]^{-1} = -\text{sgn}(\omega) \theta(|\omega| - 2\Delta) \pi \sqrt{\omega^2 - 4\Delta^2} / (2|\omega|)$  for any  $\omega$ , and perform the integral in Eq. (S24) directly. Thus, we can expand Eq. (S24) by formally adding and subtracting  $\text{Re}[\chi_{\text{SH}}^R(2\Delta, 0)]^{-1}$  from the r.h.s., integrating by parts, and evaluating the remaining integral with logarithmic accuracy using  $\text{Im}[\chi_{\text{SH}}^R(\omega, \mathbf{q})]^{-1} \simeq \pi(\xi^2 q^2 - \sqrt{\xi^4 q^4 + 4(\omega/\Delta - 2)})/4$ , we find

$$\begin{aligned} \text{Re}[\chi_{\text{SH}}^R(2\Delta, \mathbf{q})]^{-1} &= \frac{2}{\pi} \int_{2\Delta}^{\infty} d\varepsilon \frac{\varepsilon \text{Im}([\chi_{\text{SH}}^R(\varepsilon, \mathbf{q})]^{-1} - [\chi_{\text{SH}}^R(\varepsilon, 0)]^{-1})}{\varepsilon^2 - 4\Delta^2} = \frac{1}{\pi} \text{Im} \left( [\chi_{\text{SH}}^R(\varepsilon, \mathbf{q})]^{-1} - [\chi_{\text{SH}}^R(\varepsilon, 0)]^{-1} \right) \ln \frac{\varepsilon^2 - 4\Delta^2}{4\Delta^2} \Big|_{\varepsilon=2\Delta}^{\infty} \\ &- \frac{1}{\pi} \int_{2\Delta}^{\infty} d\varepsilon \ln \frac{\varepsilon^2 - 4\Delta^2}{4\Delta^2} \partial_{\varepsilon} \text{Im}([\chi_{\text{SH}}^R(\varepsilon, \mathbf{q})]^{-1} - [\chi_{\text{SH}}^R(\varepsilon, 0)]^{-1}) \simeq \int_0^{\infty} \frac{d\delta}{4} \left[ \frac{1}{\sqrt{\xi^4 q^4/4 + \delta}} - \frac{1}{\sqrt{\delta}} \right] \ln \delta = \xi^2 q^2 \ln \frac{e^{1/2}}{\xi q} + \mathcal{O}(\xi^2 q^2). \end{aligned} \quad (\text{S25})$$

In the first line here we used the fact that the imaginary part saturates to a constant at large frequency, independent of momentum. Our simple estimation in Eq. (S25) is not sufficient to fully determine the numerical factor under the logarithm. A slightly more careful calculation of the sub-leading term can be done as follows: we first subtract the leading order result  $\xi^2 q^2 \ln \frac{e^{1/2}}{\xi q}$  from both sides of the exact relation

$$\text{Re}[\chi_{\text{SH}}^R(2\Delta, \mathbf{q})]^{-1} = -\frac{1}{\pi} \int_0^\infty d\delta \ln[\delta(1+\delta/4)] \partial_\delta \text{Im} \left( [\chi_{\text{SH}}^R(2\Delta + \Delta\delta, \mathbf{q})]^{-1} - [\chi_{\text{SH}}^R(2\Delta + \Delta\delta, 0)]^{-1} \right). \quad (\text{S26})$$

Then we differentiate both sides with respect to  $\xi^2 q^2$  and take the limit  $q \rightarrow 0$ . The resulting expression gives us the coefficient  $\#$  in the expansion  $\text{Re}[\chi_{\text{SH}}^R(2\Delta, \mathbf{q})]^{-1} \approx \xi^2 q^2 \ln \frac{e^{1/2}}{\xi q} + c_2 \xi^2 q^2 + \mathcal{O}(\xi^4 q^4)$  as

$$c_2 = -\frac{1}{\pi} \int_0^{+\infty} \frac{d\delta \ln[\delta(1+4\delta)]}{\delta(\delta+2)^3(\delta+4)} \left\{ (\delta+4)(\delta(\delta+4)-4) E\left(\frac{\delta}{\delta+4}\right) - 4(\delta^2-4) K\left(\frac{\delta}{\delta+4}\right) \right\} \approx \frac{0.606}{\pi}. \quad (\text{S27})$$

Therefore, we finally obtain

$$\text{Re}[\chi_{\text{SH}}^R(2\Delta, \mathbf{q})]^{-1} = \xi^2 q^2 \ln \frac{e^{c_1}}{\xi q} + \mathcal{O}(\xi^4 q^4), \quad c_1 \equiv 1/2 + c_2 \approx 0.693. \quad (\text{S28})$$

The frequency dependence for  $\omega > 2\Delta$  can be now obtained in a similar way: we add and subtract  $\text{Re}[\chi_{\text{SH}}^R(2\Delta, \mathbf{q})]^{-1}$  from the r.h.s. of Eq. (S24), and once more use the asymptotic expression for  $\text{Im}[\chi_{\text{SH}}^R(2\Delta, \mathbf{q})]^{-1}$  given above. The result of this integration is given in the paragraph above Eq. (7) in the main text.

### LATE-TIME SH RESPONSE AT FIXED MOMENTUM

Let us consider the FT of the retarded SH susceptibility

$$\chi_{\text{SH}}^R(t, \mathbf{q}) = \int_{-\infty}^{+\infty} \frac{d\omega}{2\pi} e^{-i\omega t} \chi_{\text{SH}}^R(\omega, \mathbf{q}), \quad (\text{S29})$$

for  $t > 0$ . Given that  $\chi_{\text{SH}}(z, \mathbf{q})$  has only branch cuts on the physical sheet, we can rewrite the integral as follows

$$\chi_{\text{SH}}^R(t, \mathbf{q}) = \frac{2}{\pi} \int_{2\Delta}^{+\infty} d\omega \sin(\omega t) \text{Im} \chi_{\text{SH}}^R(\omega, \mathbf{q}) = -\frac{1}{\pi} \text{Re} \int_{2\Delta}^{+\infty} d\omega (e^{i\omega t} - e^{-i\omega t}) \chi_{\text{SH}}^R(\omega, \mathbf{q}). \quad (\text{S30})$$

For the first term, we can rotate the contour of integration counter-clockwise by  $\pi/2$  into the upper half-plane. Clearly, this is allowed because  $\chi_{\text{SH}}(z)$  does not contain non-analyticities there, and it does not grow exponentially. For the second term, we can rotate the contour clockwise by  $\pi/2$  into the unphysical Riemann sheet where the appropriate analytic continuation,  $\chi_{\text{SH}}^\downarrow(z)$ , is used. As a result, we obtain

$$\chi_{\text{SH}}^R(t, \mathbf{q}) = \text{Im} \left\{ e^{2i\Delta t} \int_0^{+\infty} \frac{dy}{\pi} e^{-ty} \chi_{\text{SH}}(2\Delta + iy, \mathbf{q}) + e^{-2i\Delta t} \int_0^{+\infty} \frac{dy}{\pi} e^{-ty} \chi_{\text{SH}}^\downarrow(2\Delta - iy, \mathbf{q}) \right\} + 2 \text{Im} [Z_{\mathbf{q}} e^{-i\omega_{\mathbf{q}} t}] \theta(\text{Re} \omega_{\mathbf{q}} - 2\Delta). \quad (\text{S31})$$

The second term here corresponds to the possibility of encountering a pole with complex frequency  $\omega_{\mathbf{q}}$  on the unphysical sheet while rotating the contour. The first term can be estimated by expanding  $\chi_{\text{SH}}(2\Delta + iy)$  and  $\chi_{\text{SH}}^\downarrow(2\Delta - iy)$  in powers of  $y$ . By construction,  $\chi_{\text{SH}}(2\Delta, \mathbf{q}) = \chi_{\text{SH}}^\downarrow(2\Delta, \mathbf{q})$  and real, and thus, the  $\sim 1/t$  term vanishes. On the other hand, we have

$$\lim_{y \rightarrow 0^+} \partial_y \chi_{\text{SH}}^\downarrow(2\Delta - iy, \mathbf{q}) = \lim_{\substack{y \rightarrow 0^+ \\ \omega \rightarrow 2\Delta^+}} \partial_y \chi_{\text{SH}}^\downarrow(\omega - iy, \mathbf{q}) = -i \lim_{\omega \rightarrow 2\Delta^+} \partial_\omega \chi_{\text{SH}}^\downarrow(\omega, \mathbf{q}) = -i \lim_{\omega \rightarrow 2\Delta^+} \partial_\omega \chi_{\text{SH}}^R(\omega, \mathbf{q}). \quad (\text{S32})$$

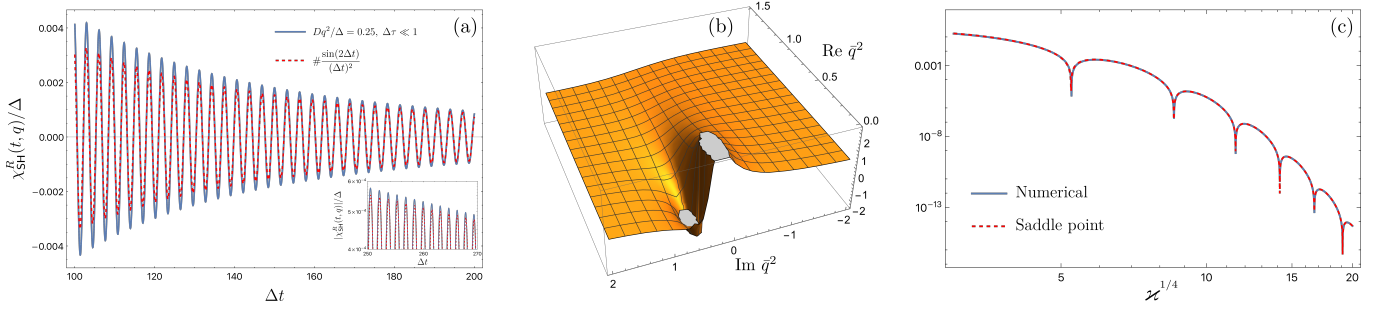

FIG. S1. (a) Oscillations of  $\chi_{\text{SH}}^R(t, \mathbf{q})$  in the time domain for  $Dq^2/\Delta = 0.25$  ( $\xi q = 0.5$ ), in a dirty limit  $\Delta\tau \ll 1$ . The red dashed line is the approximation with the first term of Eq. (S33), where the derivative is evaluated numerically without any fitting parameters. The inset is  $|\chi_{\text{SH}}^R(t, \mathbf{q})|/\Delta$  on a log-log scale. The decay  $\sim 1/t^2$  and the frequency of oscillations  $2\Delta$  are clearly seen. (b) Imaginary part of  $\chi_{\text{SH}}^R(\omega, \mathbf{q})$  as a function of complex  $\bar{q}^2$  for  $\omega/\Delta = 2.2$ . (c) Solid blue curve shows the absolute value of the l.h.s. of Eq. (S44) for  $\Delta t = 16.5$ , as a function of  $\kappa$ . The red dashed curve is the approximation shown on the r.h.s. of Eq. (S44).

In the same way, we find  $\lim_{y \rightarrow 0^+} \partial_y \chi_{\text{SH}}(2\Delta + iy, \mathbf{q}) = i \lim_{\omega \rightarrow 2\Delta^+} \partial_\omega \chi_{\text{SH}}^R(\omega, \mathbf{q})$ , and thus

$$\chi_{\text{SH}}^R(t, \mathbf{q}) \approx -\frac{2 \sin(2\Delta t)}{\pi t^2} \lim_{\omega \rightarrow 2\Delta^+} \partial_\omega \text{Im} \chi_{\text{SH}}^R(\omega, \mathbf{q}) + 2 \text{Im} [Z_{\mathbf{q}} e^{-i\omega_{\mathbf{q}} t}] \theta(\text{Re} \omega_{\mathbf{q}} - 2\Delta), \quad (\text{S33})$$

This result is given in Eq. (11) of the main text. We note that Eq. (S33) is general and does not require the dirty limit  $\Delta\tau \ll 1$ . The only details needed are the characteristics of the pole ( $\omega_{\mathbf{q}}$ ,  $Z_{\mathbf{q}}$ ), and the derivative of the imaginary part of  $\chi^R$  at  $2\Delta$ . Note that the first term in Eq. (S33) is exactly what one would obtain by integrating Eq. (S30) by parts twice. The second term, however, would be missed this way. The agreement between Eq. (S33) and the numerical result is shown in Fig. S1(a).

### LONG-DISTANCE SH RESPONSE AT FIXED FREQUENCY

We consider the following FT transform

$$\chi_{\text{SH}}^R(\omega, \mathbf{r}) = \int \frac{d^d q}{(2\pi)^d} e^{i\mathbf{q} \cdot \mathbf{r}} \chi_{\text{SH}}^R(\omega, \mathbf{q}), \quad (\text{S34})$$

for  $\omega > 0$ . For simplicity, let us consider a  $d = 3$  case. The integral over the angles is trivial and leads to

$$\chi_{\text{SH}}^R(\omega, \mathbf{r}) = \frac{1}{2\pi^2 r} \int_0^{+\infty} dq q \sin(qr) \chi_{\text{SH}}^R(\omega, q) = -\frac{i}{8\pi^2 r \xi^2} \int_0^{+\infty} d(\bar{q}^2) (e^{i\bar{q}\bar{r}} - e^{-i\bar{q}\bar{r}}) \chi_{\text{SH}}^R(\omega, \bar{q}). \quad (\text{S35})$$

Here we are using the same notation as in the main text:  $\bar{q} = \xi q$ , and  $\bar{r} = r/\xi$ . In order to extract the leading oscillatory contribution to this integral, we need to investigate the behavior of  $\chi_{\text{SH}}^R(\omega, \bar{q})$  in the complex plane of  $\bar{q}$ . We note that  $\chi_{\text{SH}}^R$  is a function of  $\bar{q}^2$  only, so we will promote  $\bar{q}^2$  to a complex variable. Numerical evaluation suggests that  $\chi_{\text{SH}}^R$  has a pole  $\bar{q}^2 = \bar{q}_\omega^2$  in the upper half-plane of  $\bar{q}^2$ , i.e.  $\text{Re} \bar{q}_\omega^2 > 0$  and  $\text{Im} \bar{q}_\omega^2 > 0$  provided  $\omega > 2\Delta$ , see Fig. S1(b). Moreover, there are no other non-analyticities in the half-plane  $\text{Re} \bar{q}^2 > 0$ . The properties of this pole in the dirty limit  $\Delta\tau \ll 1$  are discussed in the main text (see Eq. (10)).

This analytic structure suggests rotating the contours of integration to the imaginary axis in the complex  $\bar{q}^2$ -plane so that in the first term in Eq. (S35) we have  $\bar{q}^2 = \rho e^{i\pi/2}$ , and  $\bar{q}^2 = \rho e^{-i\pi/2}$  in the second term. This results in

$$\chi_{\text{SH}}^R(\omega, \mathbf{r}) = \frac{1}{4\pi^2 r \xi^2} \int_0^{+\infty} d\rho e^{-\bar{r}\sqrt{\rho/2}} \text{Re} \left\{ e^{i\bar{r}\sqrt{\rho/2}} \chi_{\text{SH}}^R(\omega, \bar{q}^2 \rightarrow i\rho) \right\} + \frac{\tilde{Z}_\omega}{4\pi r \xi^2} e^{i\bar{q}_\omega \bar{r}} \theta(\text{Re} \bar{q}_\omega^2), \quad (\text{S36})$$

where the last term originates from the pole. First, we note that the first term in Eq. (S36) is purely real, and thus,  $\text{Im} \chi_{\text{SH}}^R(\omega, \mathbf{r})$  only has a contribution from the pole. This is our result in Eq. (13) of the main text for 3D. Next, if we

expand  $\chi_{\text{SH}}^R(\omega, \bar{q}^2 \rightarrow i\rho)$  in the first term in Eq. (S36) in powers of  $\rho$  and integrate term by term, then we find that all terms in the series vanish identically. From numerical analysis, we find that the first term decays as  $\sim 1/r^3$  and contains no oscillations. Thus, the full asymptotic expression reads as

$$\chi_{\text{SH}}^R(\omega, \mathbf{r}) \approx \frac{\tilde{Z}_\omega}{4\pi r \xi^2} e^{iq_\omega \bar{r}} \theta(\text{Re } \bar{q}_\omega^2) + \mathcal{O}(1/r^3, \text{ non-oscillatory}) . \quad (\text{S37})$$

We emphasize that this expression is valid in 3D for arbitrary  $\Delta\tau$ . In the dirty limit  $\Delta\tau \ll 1$ , we can use Eq. (10) of the main text and obtain

$$\text{Im } \chi_{\text{SH}}^R(\omega, \mathbf{r}) \simeq \frac{\sin(r/\xi_\omega) e^{-\frac{r}{\xi_\omega}}}{\pi r \xi^2 \ln \frac{e^{4c_1}}{\bar{\omega}-2}} , \quad \frac{\xi_\omega}{\xi} = \frac{\ln^{1/2} \frac{e^{4c_1}}{\bar{\omega}-2}}{\sqrt{\pi}(\bar{\omega}-2)^{1/4}} . \quad (\text{S38})$$

At  $\omega = 2\Delta$ , one can evaluate the integral directly as follows

$$\chi_{\text{SH}}^R(\omega = 2\Delta, \mathbf{r}) \approx \frac{1}{2\pi^2 r \xi^2} \int_0^{+\infty} dq \frac{\sin(qr)}{q \ln \frac{e^{c_1}}{\xi q}} \approx \frac{1}{4\pi r \xi^2 \ln \frac{e^{c_1}}{\xi}} , \quad d = 3 . \quad (\text{S39})$$

Note that Eq. (S38) and Eq. (S39) smoothly connect at  $r \approx \xi_\omega$ . Thus, Eq. (S38) describes the oscillatory asymptotic at  $r \gg \xi_\omega$  which becomes Eq. (S39) in the range  $\xi \ll r \ll \xi_\omega$ .

The analysis of the 2D case is similar. The only difference is that the Bessel function  $J_0(qr)$  should be used instead of  $\sin(qr)/qr$  in Eq. (S35). Consequently, the Bessel function is decomposed as a sum of the Hankel functions  $H_0^{(1/2)}(x)$  of the first and second kind. One then can use the fact that  $H_0^{(1/2)}(x)$  decays in the first (fourth) quadrant of the complex plane, enabling rotations of the integration contours as in the 3D case. The results are given in Eq. (13,14) of the main text.

## LATE-TIME AND LONG-DISTANCE SH RESPONSE

Finally, let us consider the FT with respect to both momentum and frequency

$$\chi_{\text{SH}}^R(t, \mathbf{r}) = \frac{2}{\pi} \int_{2\Delta}^{+\infty} d\omega \sin(\omega t) \text{Im } \chi_{\text{SH}}^R(\omega, \mathbf{r}) = -\frac{1}{\pi} \text{Re} \int_{2\Delta}^{+\infty} d\omega (e^{i\omega t} - e^{-i\omega t}) \chi_{\text{SH}}^R(\omega, \mathbf{r}) . \quad (\text{S40})$$

Let us first consider the 3D case first. To this end, we can use our result in Eq. (S38). We first introduce a dimensionless integration variable  $z$  as  $\omega = 2\Delta + z/t$ . Then we assume (and verify later) that  $\Delta t \gg 1$  is much greater than the typical values of  $|z|$  that are important for the integral. Under this assumption, the logarithm of  $\omega/2\Delta - 1$  in the expression for  $\xi_\omega$  can be replaced with the logarithm of  $\Delta t$ . This allows us to write

$$\chi_{\text{SH}}^R(t, \mathbf{r}) \approx -\frac{1}{\pi^2 \xi^2 r t \ln(\Delta t)} \text{Re} \left( e^{-2i\Delta t} \left[ I((1+i)\varkappa^{1/4}) - I((1-i)\varkappa^{1/4}) \right] \right) . \quad (\text{S41})$$

Here we introduced a dimensionless parameter  $\varkappa$  and a function of a complex variable  $I(x)$ , defined as

$$\varkappa = \frac{\pi^2 (r/\xi)^4}{\Delta t \ln^2(\Delta t)} , \quad I(x) = \int_0^{+\infty} dz \exp \left\{ -iz - xz^{1/4} \right\} . \quad (\text{S42})$$

We will evaluate  $I((1 \pm i)\varkappa^{1/4})$  by the stationary phase method assuming  $\varkappa \gg 1$ . For  $x = (1-i)\varkappa^{1/4}$ , the saddle point is given by  $z_* = \frac{\varkappa^{1/3}}{4} e^{\frac{i\pi}{3}}$ . The function in the exponential evaluated at  $z_*$  is  $-\frac{3}{4} e^{-i\pi/6} \varkappa^{1/3}$ . The remaining Gaussian integral yields

$$I((1-i)\varkappa^{1/4}) \approx \sqrt{\frac{2\pi}{3}} \varkappa^{1/6} \exp \left\{ -\frac{3}{4} e^{-i\pi/6} \varkappa^{1/3} - \frac{i\pi}{12} \right\} . \quad (\text{S43})$$

It turns out that the saddle point in  $I((1+i)\varkappa^{1/4})$  is located on the negative real axis, on top of the branch cut of  $z^{1/4}$ . Thus, it is inaccessible, and the contribution of  $I((1+i)\varkappa^{1/4})$  can be ignored. The result then reads as

$$\text{Re} \left( e^{-2i\Delta t} \left[ I((1+i)\varkappa^{1/4}) - I((1-i)\varkappa^{1/4}) \right] \right) \approx -\sqrt{\frac{2\pi}{3}} \varkappa^{1/6} e^{-\frac{3\sqrt{3}}{8}\varkappa^{1/3}} \cos \left( \frac{3}{8}\varkappa^{1/3} - 2\Delta t - \frac{\pi}{12} \right). \quad (\text{S44})$$

We demonstrate the accuracy of this approximation in Fig. S1(c). We also note that the typical  $|z|$  involved in this saddle point estimation is of the order of  $\varkappa^{1/3}$ . Therefore, for our initial assumption to be self-consistent, we need to have  $\Delta\tau \gg \varkappa^{1/3}$ , i.e.  $\Delta t \ln^{1/2} \Delta t \gg r/\xi$ . Given the  $z = 4$  dynamical scaling, the oscillations of interest occur at  $r/\xi \sim (\Delta\tau)^{1/4} \ln^{1/2} \Delta\tau \ll \Delta\tau$ , so our result is well within the regime of control.

After combining these expressions, we find

$$\chi_{\text{SH}}^R(t, \mathbf{r}) \approx \frac{\Delta}{\sqrt{3/2}\pi^{7/6}\xi^3} \times \frac{e^{-\frac{3\sqrt{3}}{8}\varkappa^{1/3}}}{(r/\xi)^{1/3}(\Delta t)^{7/6} \ln^{4/3}(\Delta t)} \cos \left( \frac{3}{8}\varkappa^{1/3} - 2\Delta t - \frac{\pi}{12} \right), \quad d = 3. \quad (\text{S45})$$

In the 2D case, the integral in Eq. (S42) contains an extra factor  $1/z^{1/8}$  which should be evaluated at the saddle point  $z_*$ . The result is given in Eq. (15) of the main text.

- 
- [1] P. W. Anderson, Theory of dirty superconductors, *J. Phys. Chem. Solid* **11**, 26 (1959).
  - [2] A. A. Abrikosov and L. P. Gor'kov, On the theory of superconducting alloys, I. The electrodynamics of alloys at absolute zero, *Sov. Phys. JETP* **8**, 1090 (1959).
  - [3] A. A. Abrikosov and L. P. Gor'kov, Superconducting alloys at finite temperatures, *Sov. Phys. JETP* **9**, 220 (1959).
  - [4] P. A. Lee and T. V. Ramakrishnan, Disordered electronic systems, *Rev. Mod. Phys.* **57**, 287 (1985).
  - [5] A. D. Mirlin, Statistics of energy levels and eigenfunctions in disordered systems, *Physics Reports* **326**, 259 (2000).
  - [6] I. O. Kulik, O. Entin-Wohlman, and R. Orbach, Pair susceptibility and mode propagation in superconductors: A microscopic approach, *J. Low Temp. Phys.* **43**, 591 (1981).
  - [7] E. Andriyakhina, P. Nosov, S. Raghu, and I. Burmistrov, Quantum fluctuations and multifractally enhanced superconductivity in disordered thin films, *J. Low Temp. Phys.*, 1 (2024).
  - [8] D. Phan and A. V. Chubukov, Following the Higgs mode across the BCS-BEC crossover in two dimensions, *Phys. Rev. B* **107**, 134519 (2023).
